# Supplementary material for: STELLA: Continual Audio-Video Pre-training with Spatio-Temporal Localized Alignment
Source: arXiv:2310.08204 source file (2024-05-28)
Supplement: Supplementary file 2 [file supplement_figure_dataset_stat.tex]

\begin{figure*}[t]
    \centering
    
    \begin{minipage}{0.48\textwidth}
    \centering
    \setlength{\tabcolsep}{-1pt}{%
    \includegraphics[width=1.0\linewidth, trim={0.0cm 0.0cm 0.0cm 0.0cm},clip]{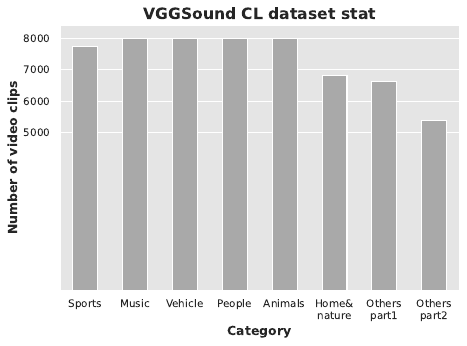}
    }
    \textbf{(a) Continual-VS statistics}
    \end{minipage}
    \hspace{0.5cm}
    \begin{minipage}{0.46\textwidth}
    \centering
    \setlength{\tabcolsep}{-1pt}{%
    \includegraphics[width=1.0\linewidth, trim={0.0cm 0.0cm 0.0cm 0.0cm},clip]{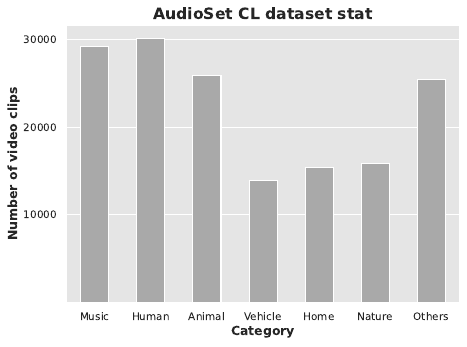}
    }
    \textbf{(b) Continual-AS statistics}
    \end{minipage}
    % \vspace{0.15in}

    \caption{\small \textbf{Stastics of Audio-Video datasets} \textbf{(a)}: We split the VGGSound into 8 tasks, where each subset dataset consists of similar amounts of video clips. 
    \textbf{(b)}: We split the AudioSet into 7 tasks. Unlike the VGGSound dataset, the number of video clips varies significantly for each task.
    }
    \label{fig:dataset_stat}
\end{figure*}
