# Supplementary material for: STELLA: Continual Audio-Video Pre-training with Spatio-Temporal Localized Alignment
Source: arXiv:2310.08204 source file (2024-05-28)
Supplement: Supplementary file 3 [file supplement_figure_no_mae.tex]

\begin{figure*}
    
    \resizebox{\linewidth}{!}{%
    \begin{tabular}{cccc}
    \includegraphics[width=0.24\linewidth]{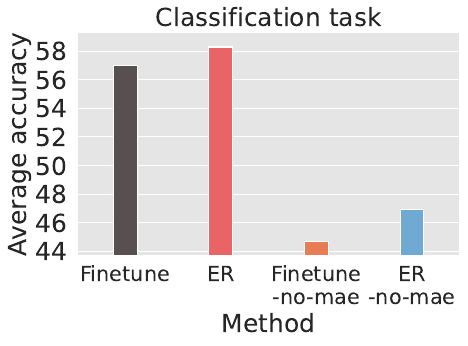}&
    \includegraphics[width=0.24\linewidth]{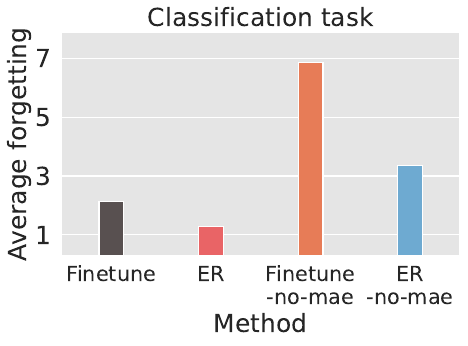}&
    \includegraphics[width=0.24\linewidth]{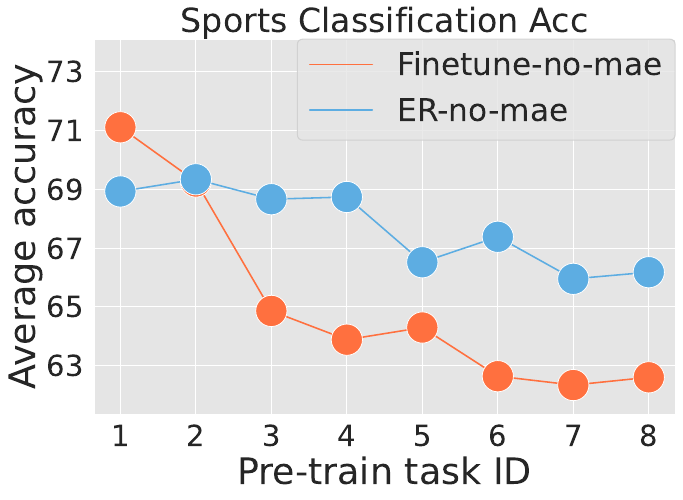}&
    \includegraphics[width=0.24\linewidth]{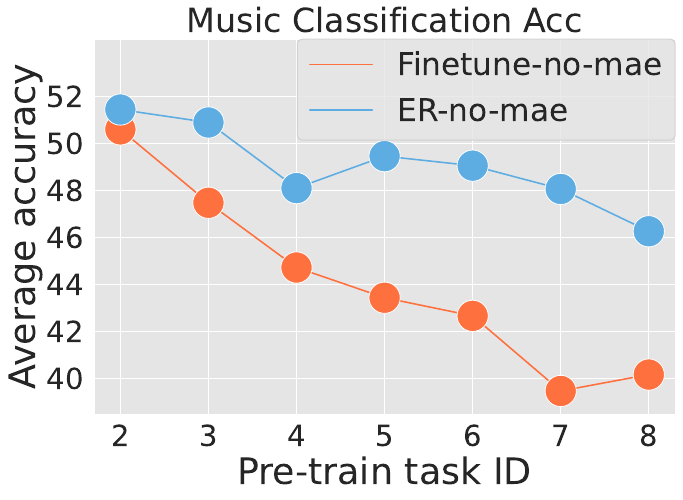}\\
        \multicolumn{2}{c}{\textbf{(a) Comparison of classification results}} &
        \multicolumn{2}{c}{\textbf{(b) Task-wise task-specific classification result}}\\
    \end{tabular}}
\vspace{-0.05in}
 \caption{\textbf{Audiovisual classification results without MAE loss term.} \textbf{(a)}: We compare the audiovisual classification results from the models with the MAE loss term (\textit{Finetune}, \textit{ER}) and the models without it (\textit{Finetune-no-mae}, \textit{ER-no-mae}). \textbf{(b)}: We visualize changes in the task-specific average classification accuracy of the sequentially pre-trained model without the MAE loss term.
 }
    \label{fig:no_mae_result}
\vspace{-0.05in}
\end{figure*}
