# Supplementary material for: STELLA: Continual Audio-Video Pre-training with Spatio-Temporal Localized Alignment
Source: arXiv:2310.08204 source file (2024-05-28)
Supplement: Supplementary file 4 [file supplement_figure_scl_ucl.tex]

\begin{figure*}[t]
    \centering
    \begin{tabular}{c}
    \includegraphics[width=1.0\linewidth]{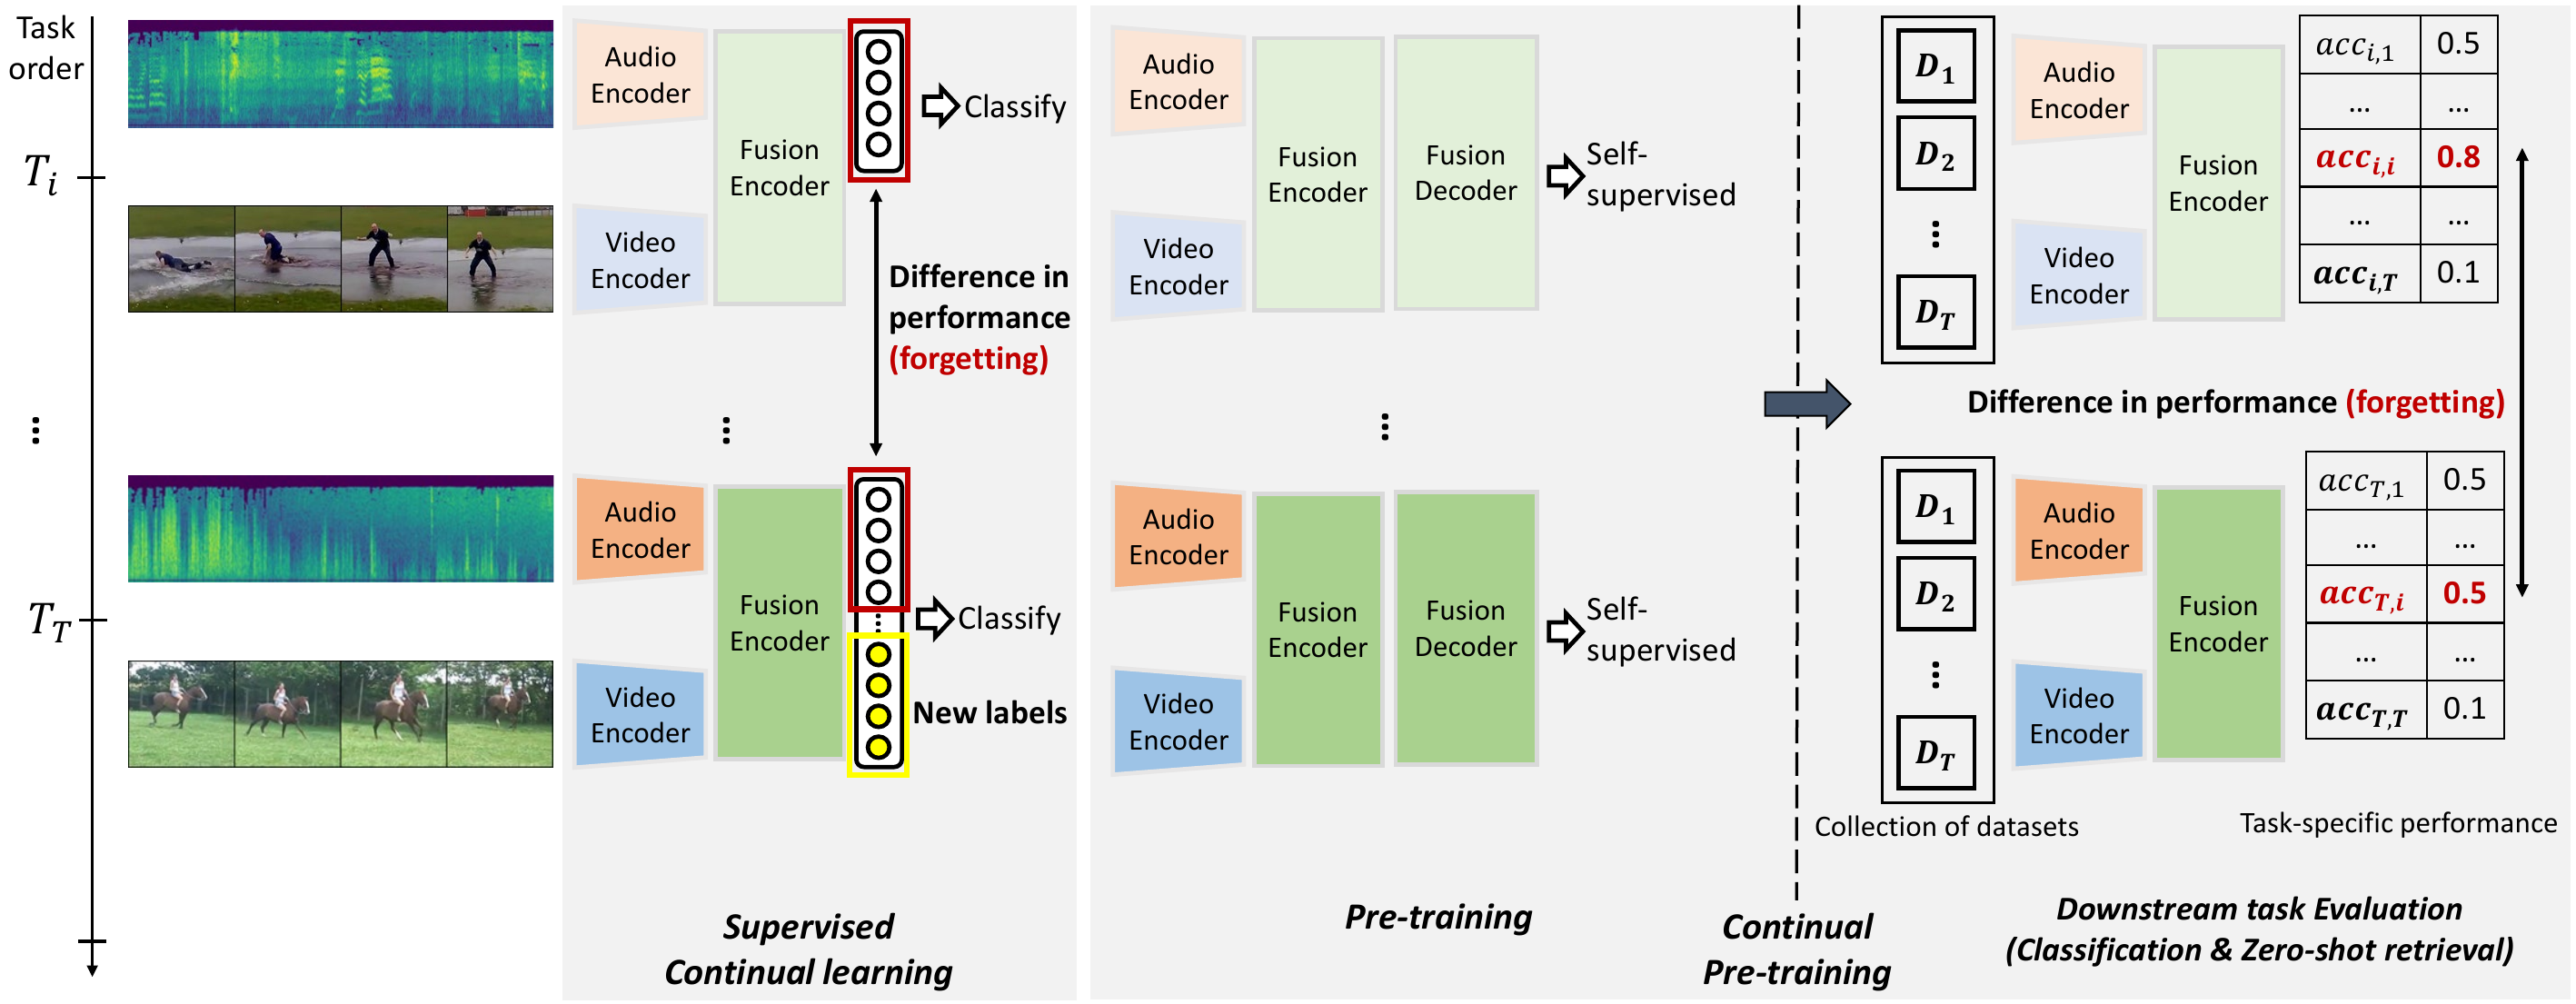}
    \end{tabular}
    \vspace{-0.15in}
    \caption{\small \textbf{Comparison with supervised continual learning and continual pre-training}: We illustrate the difference between the supervised continual learning setup and the continual pre-training setup that we used in our experiments.}
    \label{fig:scl_ucl}
\end{figure*}
