# Supplementary material for: STELLA: Continual Audio-Video Pre-training with Spatio-Temporal Localized Alignment
Source: arXiv:2310.08204 source file (2024-05-28)
Supplement: Supplementary file 5 [file supplement_table_dataset_config.tex]

\resizebox{1.0\textwidth}{!}{%
\addtolength{\tabcolsep}{-2.8pt}

\renewcommand{\tabcolsep}{3pt}
\begin{tabular}{l cccccccc ccccccc}
    \toprule
     & \multicolumn{8}{c}{VGGSound} & \multicolumn{7}{c}{AudioSet} \\
    \midrule
    {Category} & {Sports} & {Music} & {Vehicle} & {People} & {Animals} & {Home\&nature} & {Others part1} & {Others part2} & {Music} & {Human} & {Vehicle} & {Home} & {Nature} & {Others} \\
    \cmidrule{2-16}
    Train & 7737 & 8000 & 8000 & 8000 & 8000 & 6807 & 6639 & 5390 & 29144 & 30073 & 25865 & 13924 & 15373 & 15848 & 25416 \\
    Evaluate & 886 & 907 & 906 & 862 & 873 & 837 & 863 & 810 & 1188 & 1523 & 1011 & 680 & 864 & 403 & 1585 \\
    Retrieval & 119 & 288 & 139 & 209 & 317 & 92 & 85 & 104 & 130 & 145 & 126 & 103 & 81 & 42 & 175 \\
    \bottomrule
\end{tabular}}
