# Supplementary material for: STELLA: Continual Audio-Video Pre-training with Spatio-Temporal Localized Alignment
Source: arXiv:2310.08204 source file (2024-05-28)
Supplement: Supplementary file 6 [file supplement_table_forget_robust_method.tex]

\begin{wraptable}{t}{0.35\textwidth}
    \centering
    \caption{\small Retrieval result by prune methods pre-trained on VGGSound dataset.}
    \vspace{-0.1in}
    \begin{adjustbox}{width=\linewidth}
    \begin{tabular}{l cc cc}
        \toprule
        Method & \multicolumn{2}{c}{A$\rightarrow$V} & \multicolumn{2}{c}{V$\rightarrow$A} \\
        & $\mathcal{A} \uparrow$ & $\mathcal{F} \downarrow$ & $\mathcal{A} \uparrow$ & $\mathcal{F} \downarrow$ \\
        \midrule
        Random & 3.30 & 9.26 & 3.13 & 8.83 \\
        Attention & 12.18 & 6.27 & 12.08 & 6.82 \\
        \textbf{OURS} & \textbf{13.88} & \textbf{4.85} & \textbf{14.02} & \textbf{4.99}  \\
        \bottomrule
    \end{tabular}
    \end{adjustbox}
    \label{tab:forget_robust_prune_method}
\end{wraptable}
